# Supplementary material for: Computational diagnosis and risk evaluation for canine lymphoma
Source: arXiv:1305.4942 ancillary file (2014-07-03)
Supplement: Supplementary file 1 [file DataAnalysisFlowCharts.pdf]

# Supplementary materials to

# Computational diagnosis and risk evaluation for canine lymphoma

E. M. Mirkes
*Department of Mathematics, University of Leicester, Leicester, LE1 7RH, UK*

I. Alexandrakis, K. Slater, R. Tuli
*Avacta Animal Health, Unit 706, Avenue E, Thorp Arch Estate, Wetherby, LS23 7GA, UK*

A. N. Gorban[1]
*Department of Mathematics, University of Leicester, Leicester, LE1 7RH, UK*

## Flowcharts of data analysis

In this pdf file, the data analysis methods and procedures used in the paper are represented by a system of flowcharts connected by internal hyperlinks. Most flowcharts contain the legend in right top corner which explain the meaning of variables used.

*Notations*:

The variables are highlighted by italic font in all of the flowcharts.
Flowcharts use the following types of blocks:

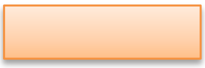 represents a process;

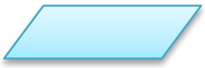 is used for data (including input data, intermediate results and outputs);

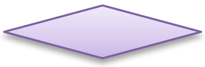 indicates a decision point or a conditional jump;

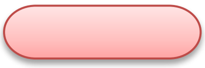 is a subprocess terminator.

[1] *E-mail address*: ag163@le.ac.uk

# General scheme of study

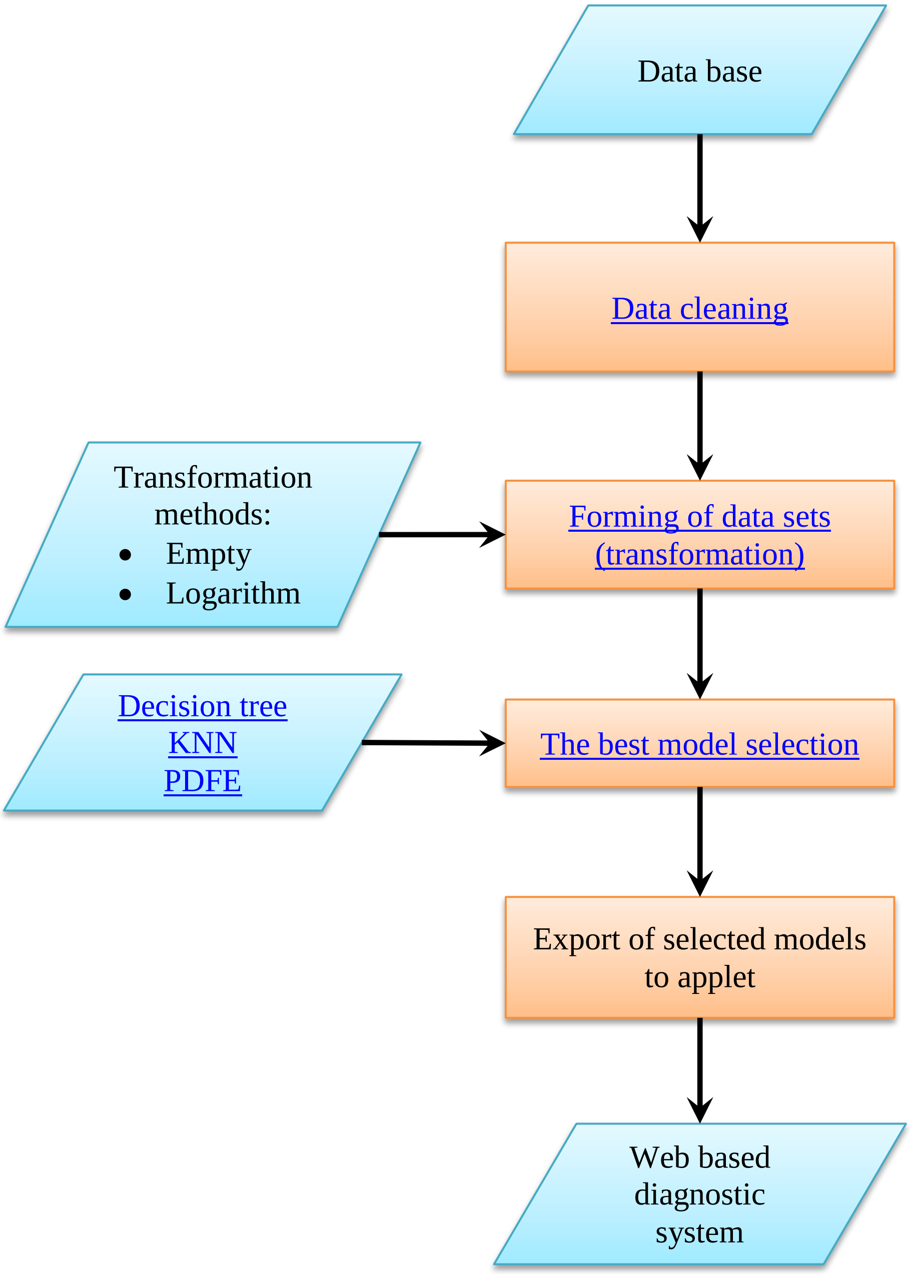

# Data cleaning

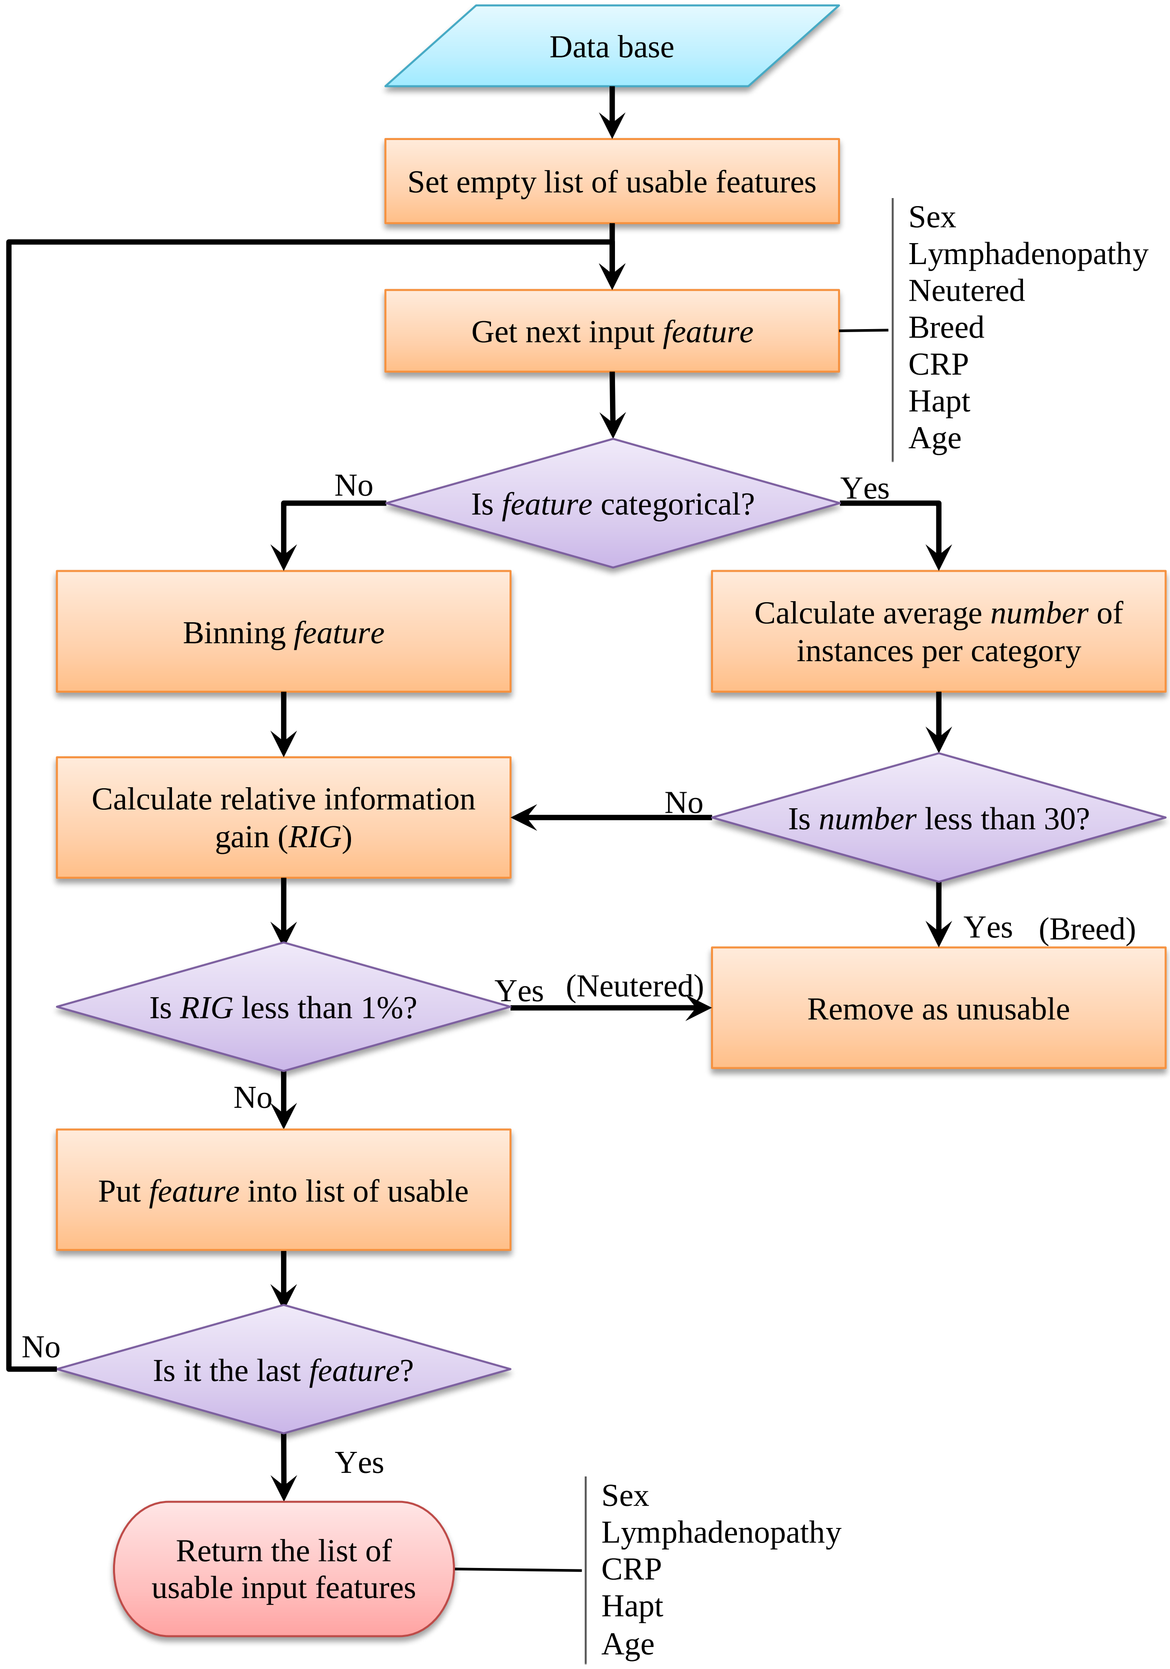

# Forming of data sets (transformation)

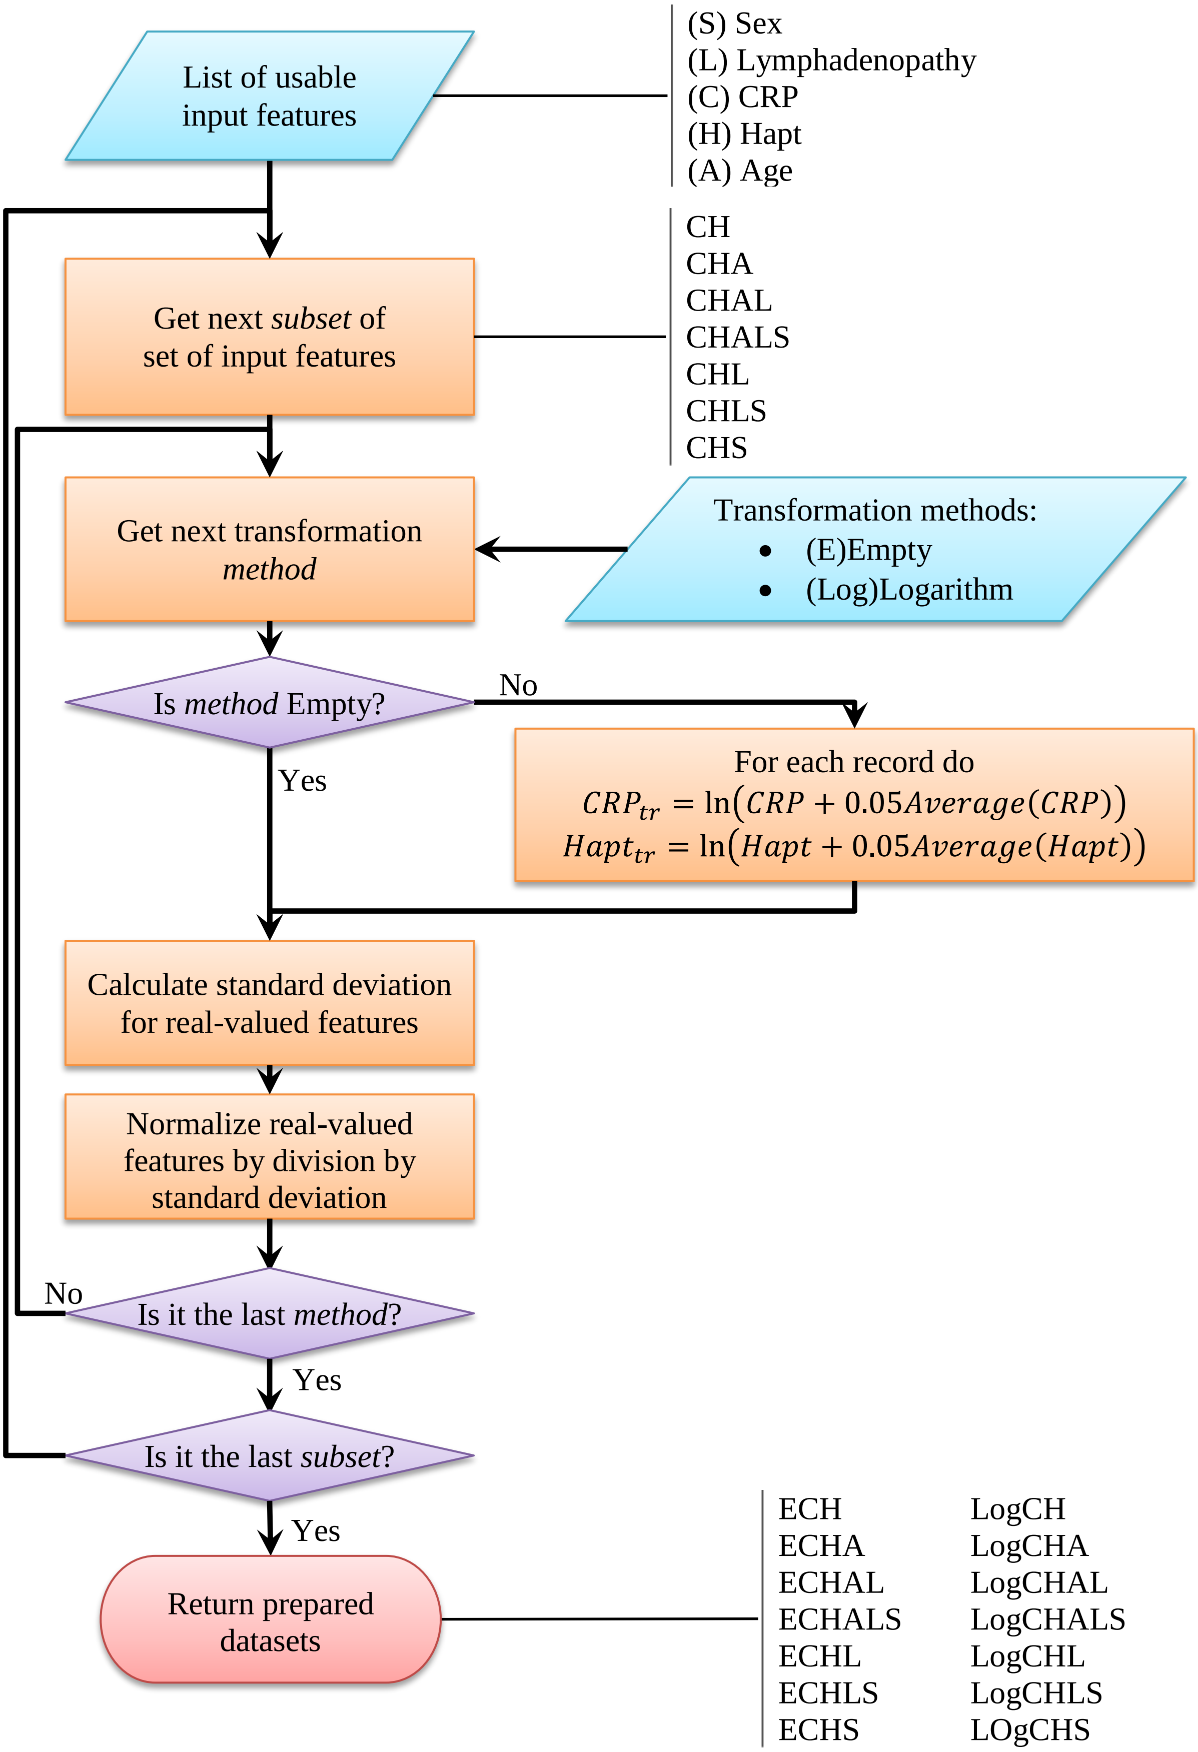

## The best model selection

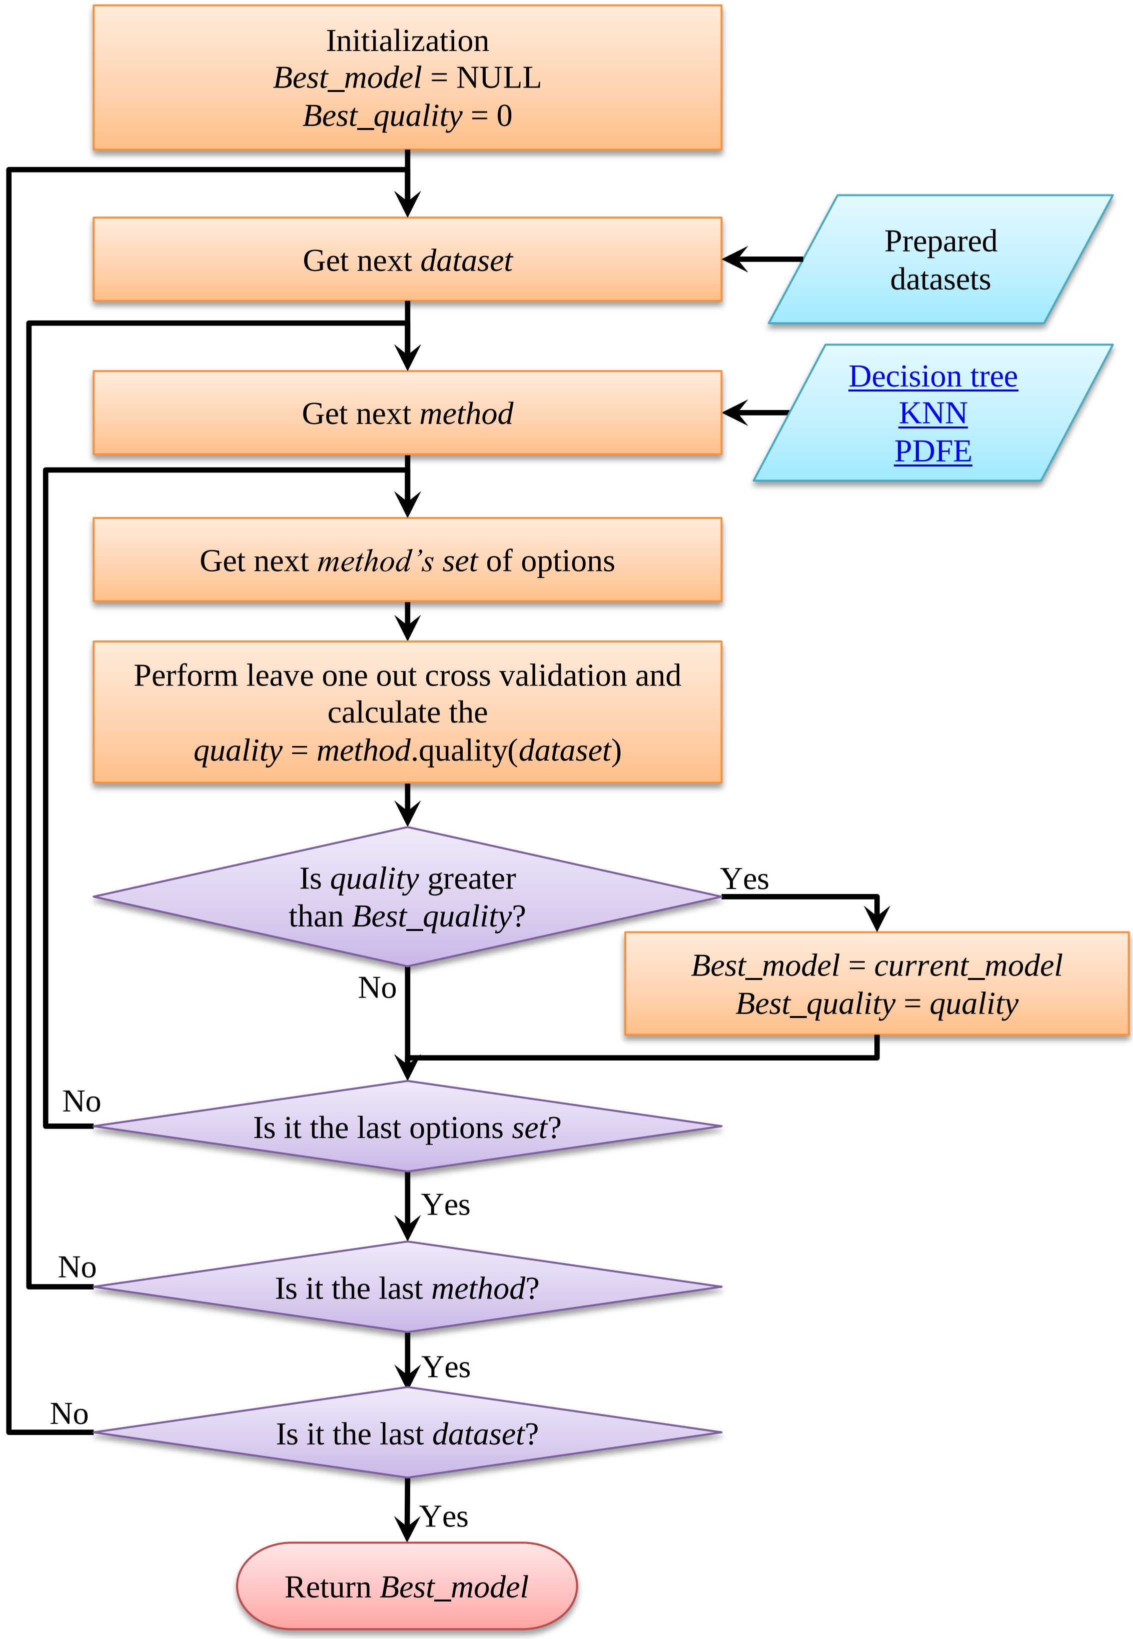

# Decision tree: quality(*Dataset*)

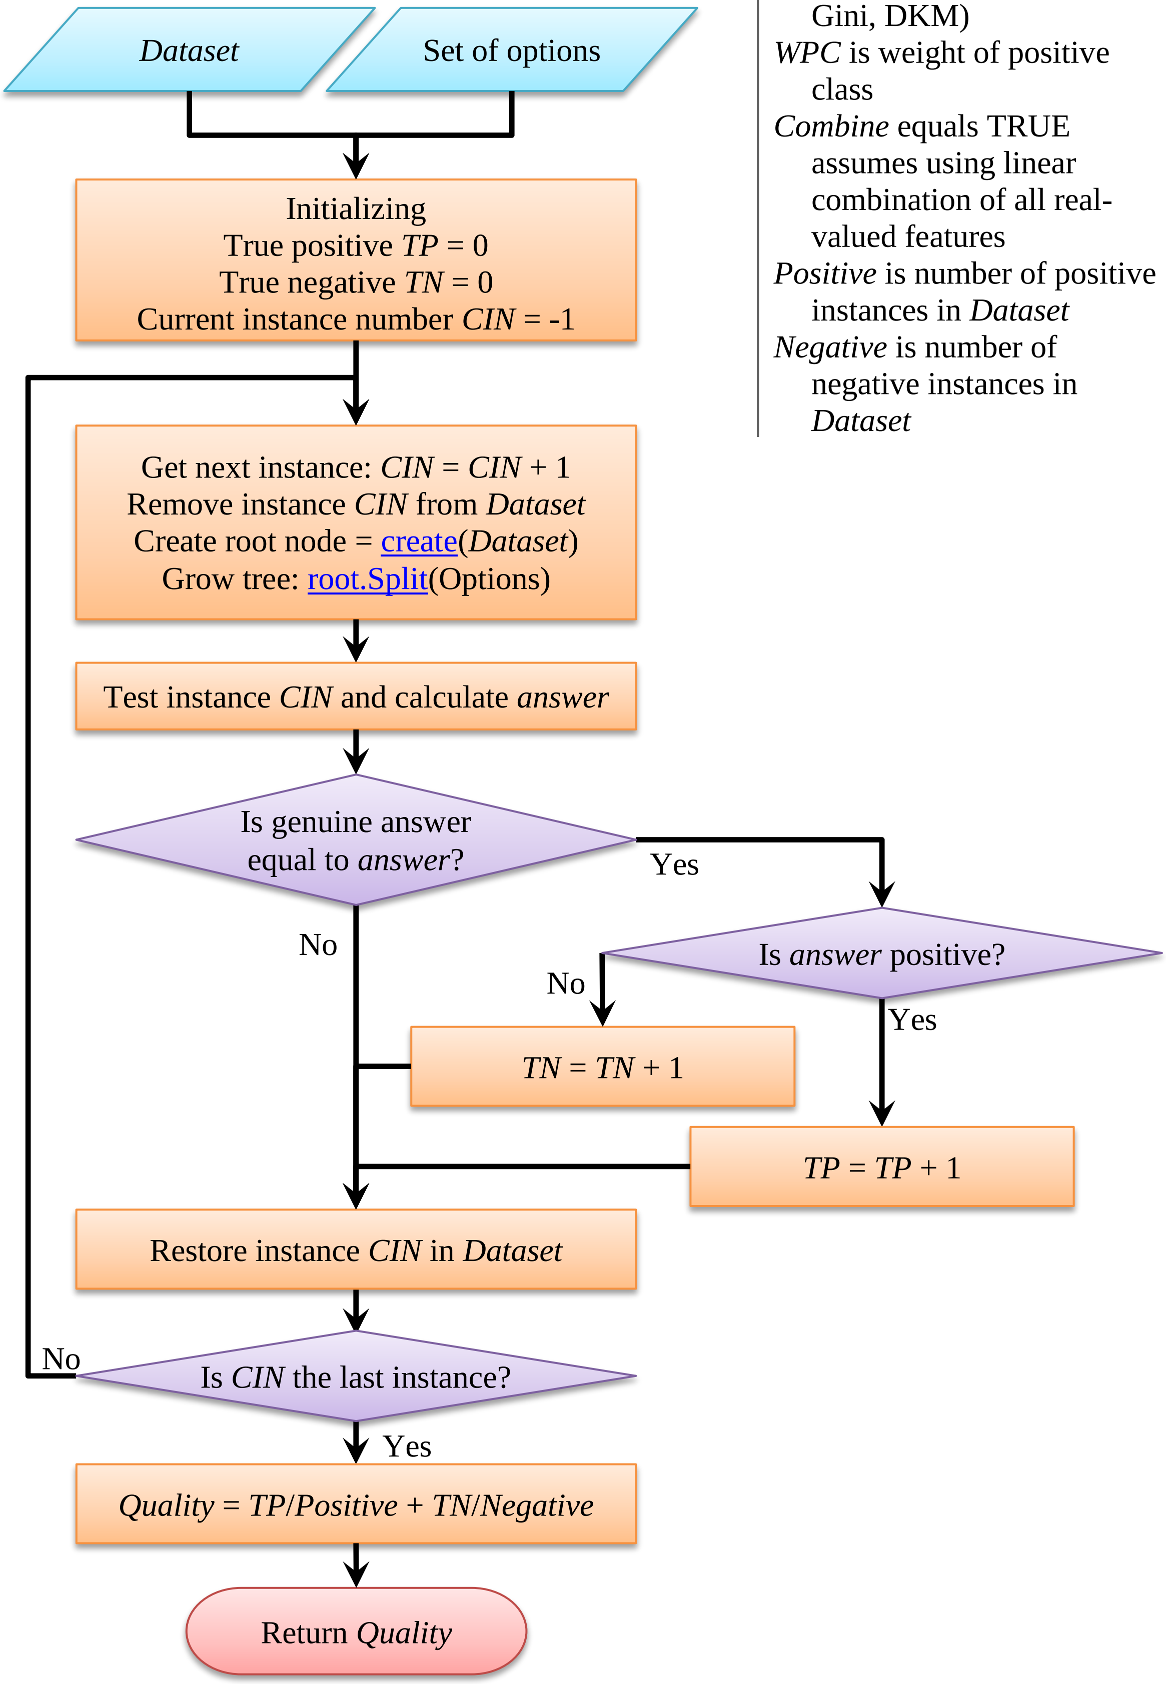


*MIL* is minimum number of instances in leaf (3-19)

*Splitting* criterion (Entropy, Gini, DKM)

*WPC* is weight of positive class

*Combine* equals TRUE assumes using linear combination of all real-valued features

*Positive* is number of positive instances in *Dataset*

*Negative* is number of negative instances in *Dataset*

# Node creation: create(*SIN*)

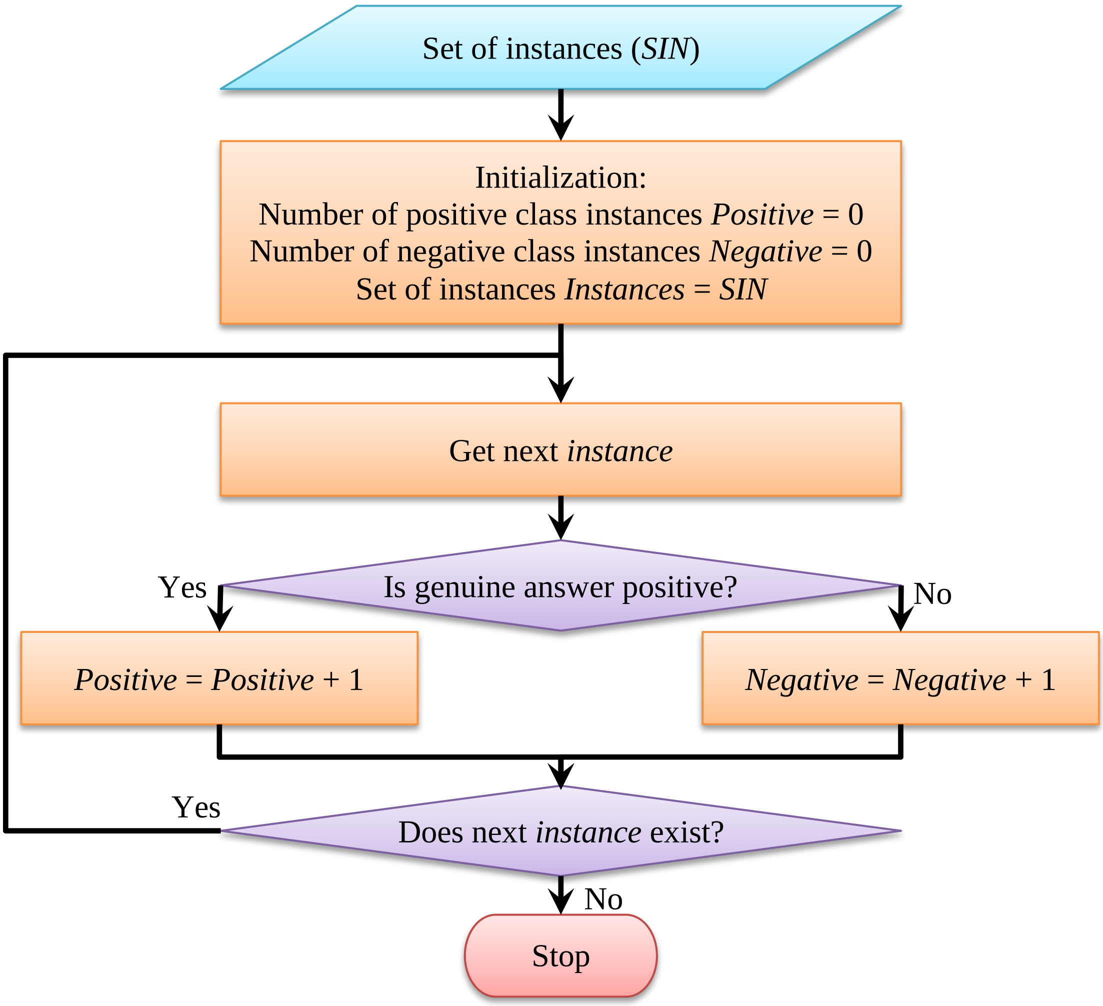

# Node splitting: Split(Options)

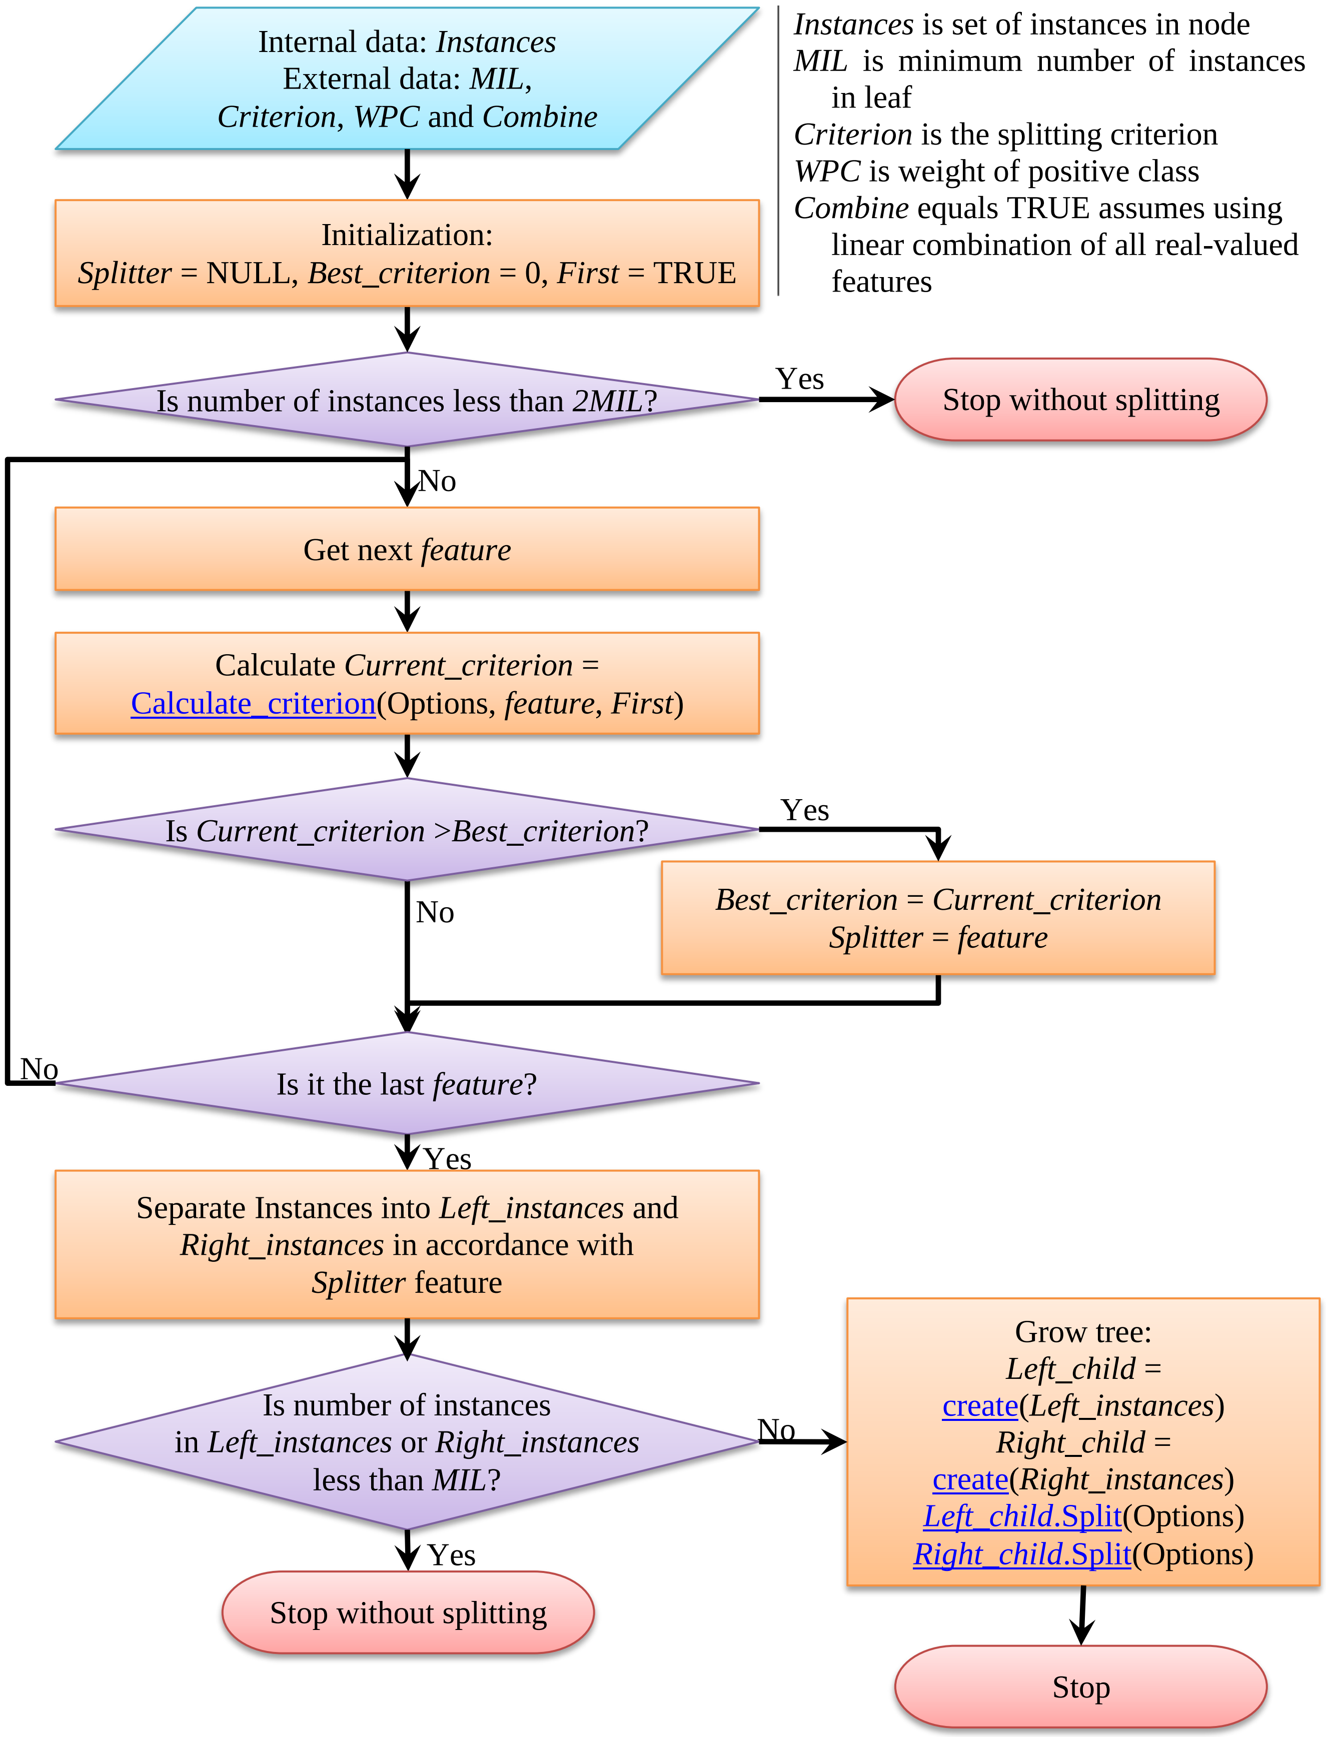

# Calculate criterion:
# Calculate_criterion(Options, *Feature*, *First*)

*Instances* is set of instances in node
*MIL* is minimum number of instances in leaf
*Criterion* is the splitting criterion
*WPC* is weight of positive class
*Combine* equals TRUE assumes using linear combination of all real-valued features
*Feature* is the feature to use
*First* is true if it is the first call for real-valued feature

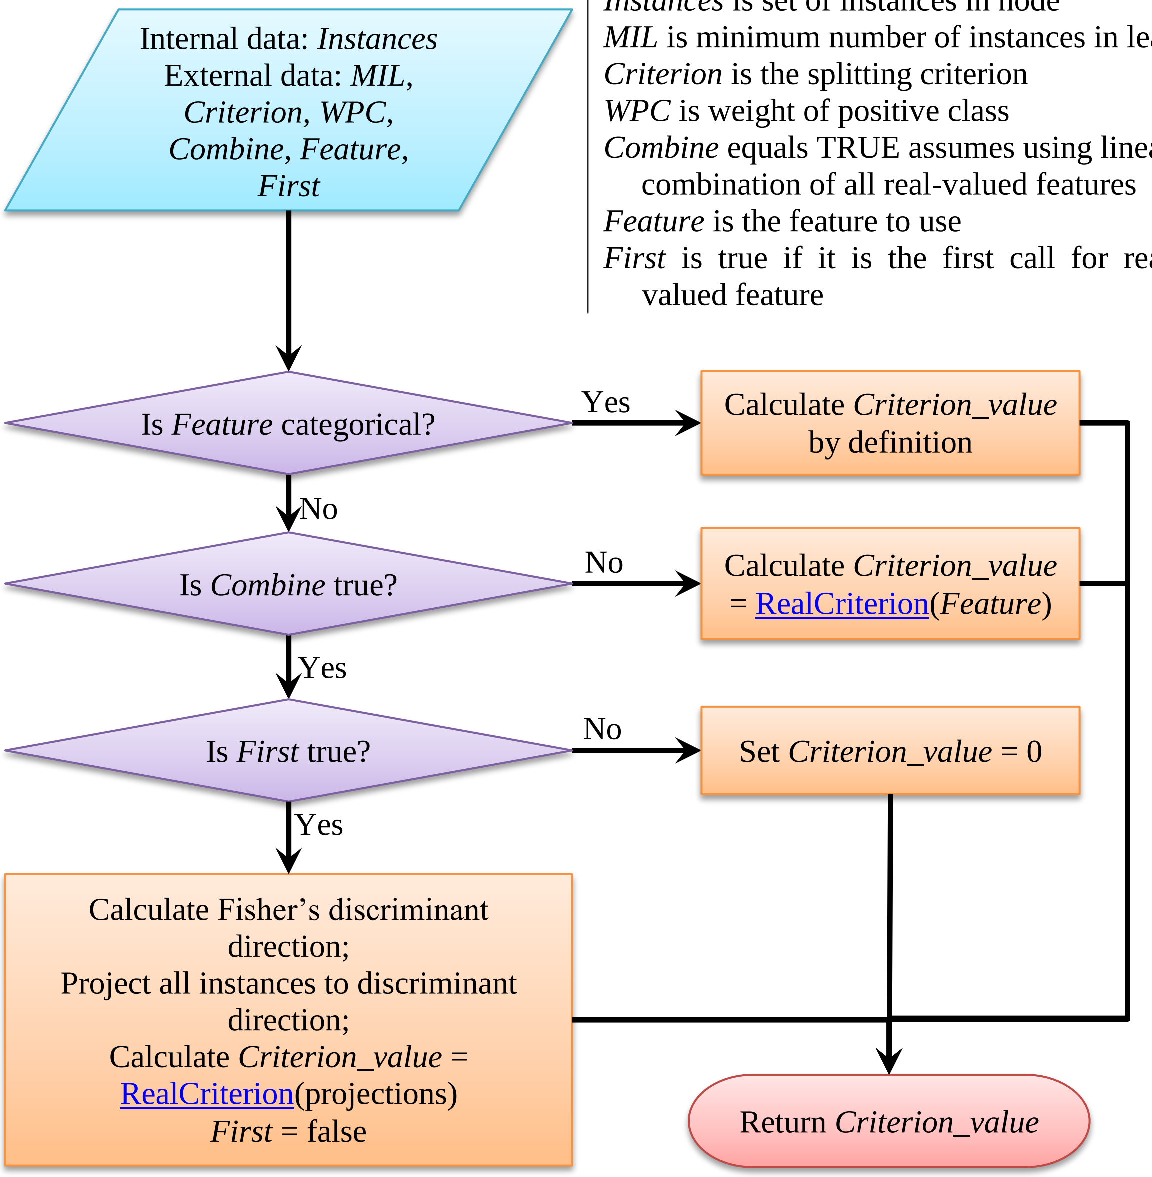

## Calculate criterion: RealCriterion(*Values*)

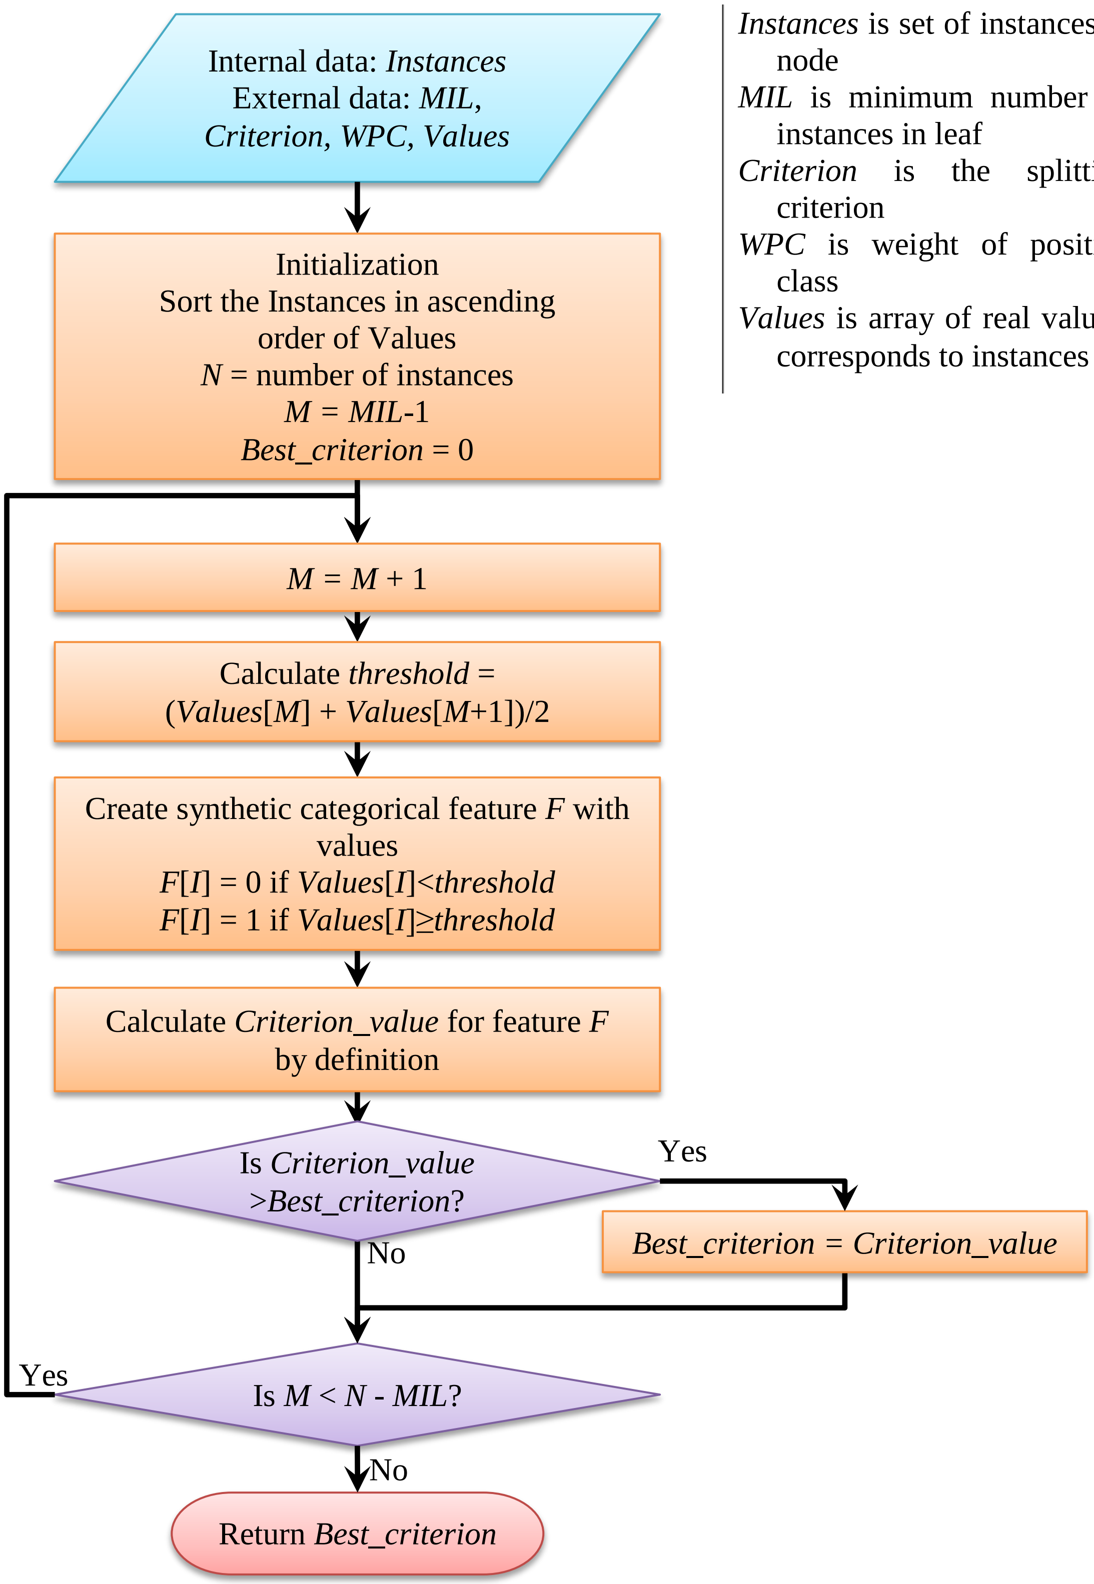


*Instances* is set of instances in node
*MIL* is minimum number of instances in leaf
*Criterion* is the splitting criterion
*WPC* is weight of positive class
*Values* is array of real values, corresponds to instances

# KNN (k nearest neighbours): quality(*Dataset*)

*Distance* (Euclidean, Fisher's, Advanced)
*K* is number of neighbours to transform distance (Fisher's and Advanced)
*Kernel* is the statistics kernel function for distance transformation (Advanced)
*k* is the number of neighbours for vote.
*Vote* is the statistics kernel function for vote
*Positive* is number of positive instances in *Dataset*
*Negative* is number of negative instances in *Dataset*

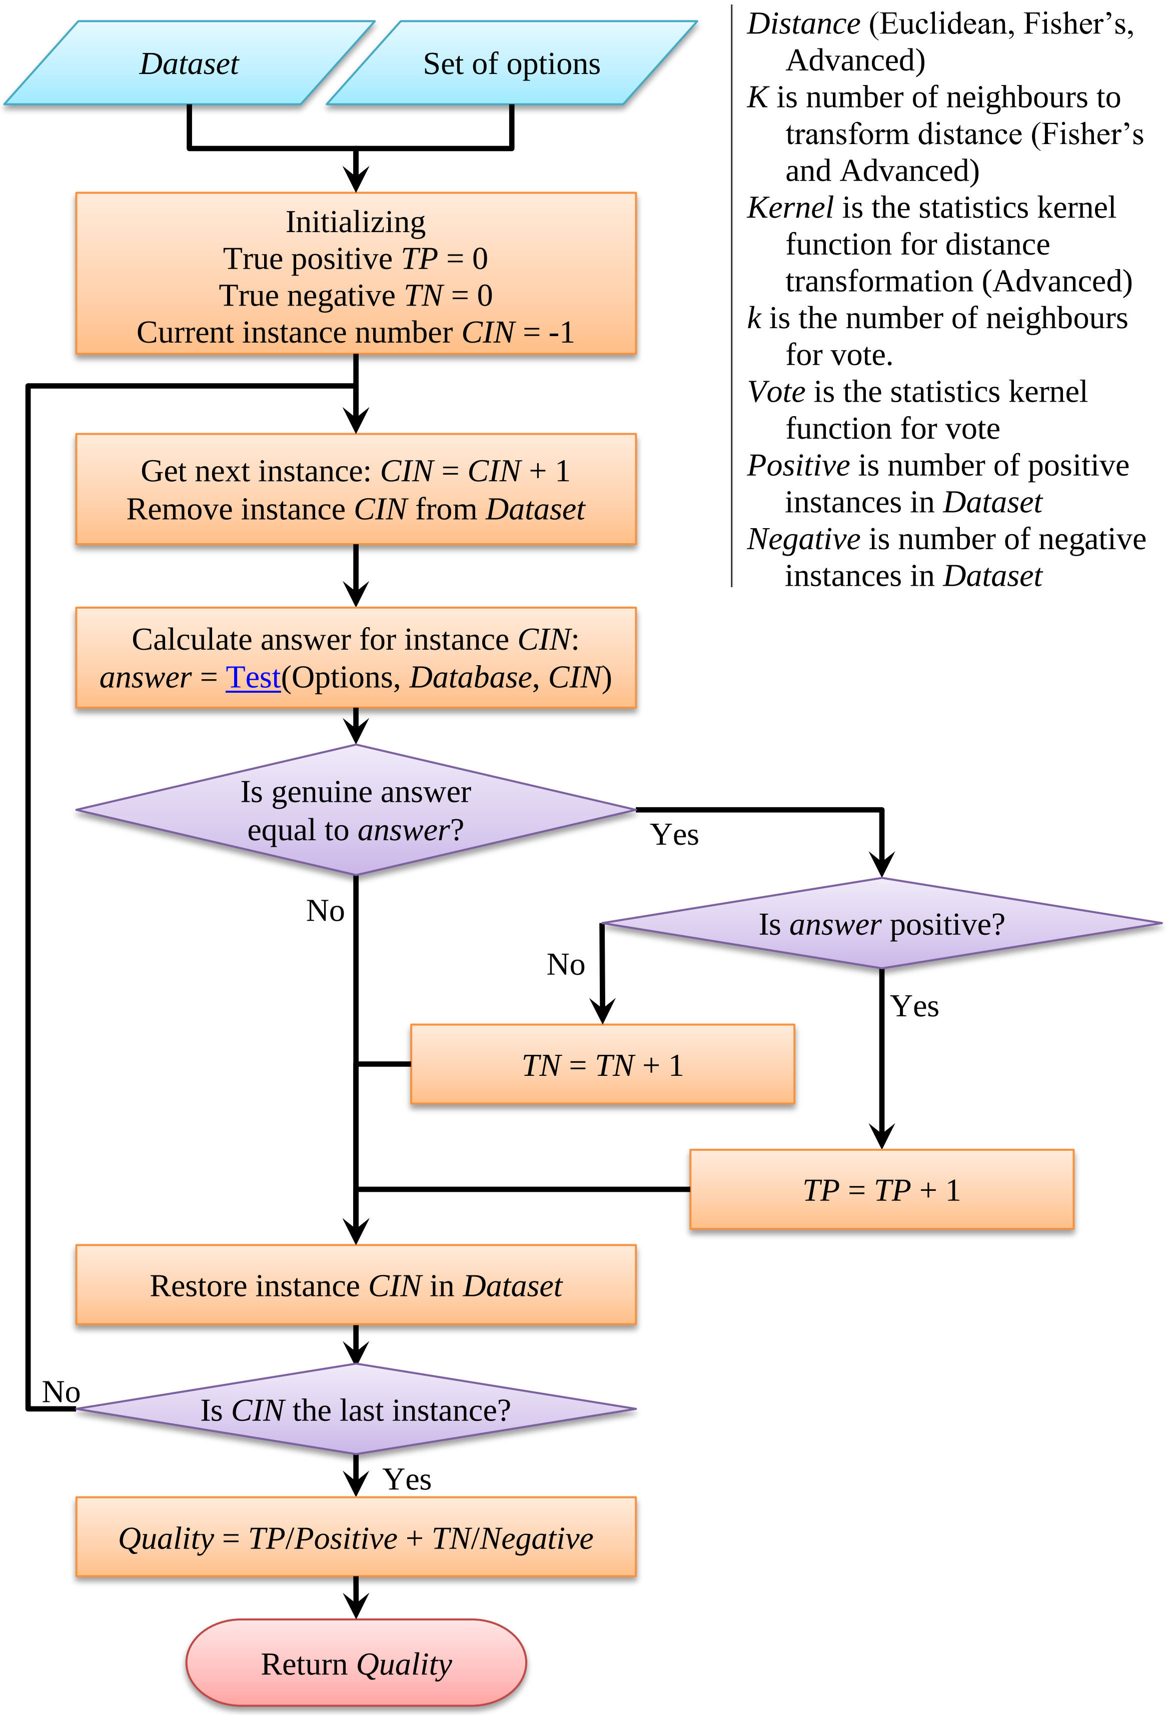

# KNN Test(Options, *Database*, *CIN*)

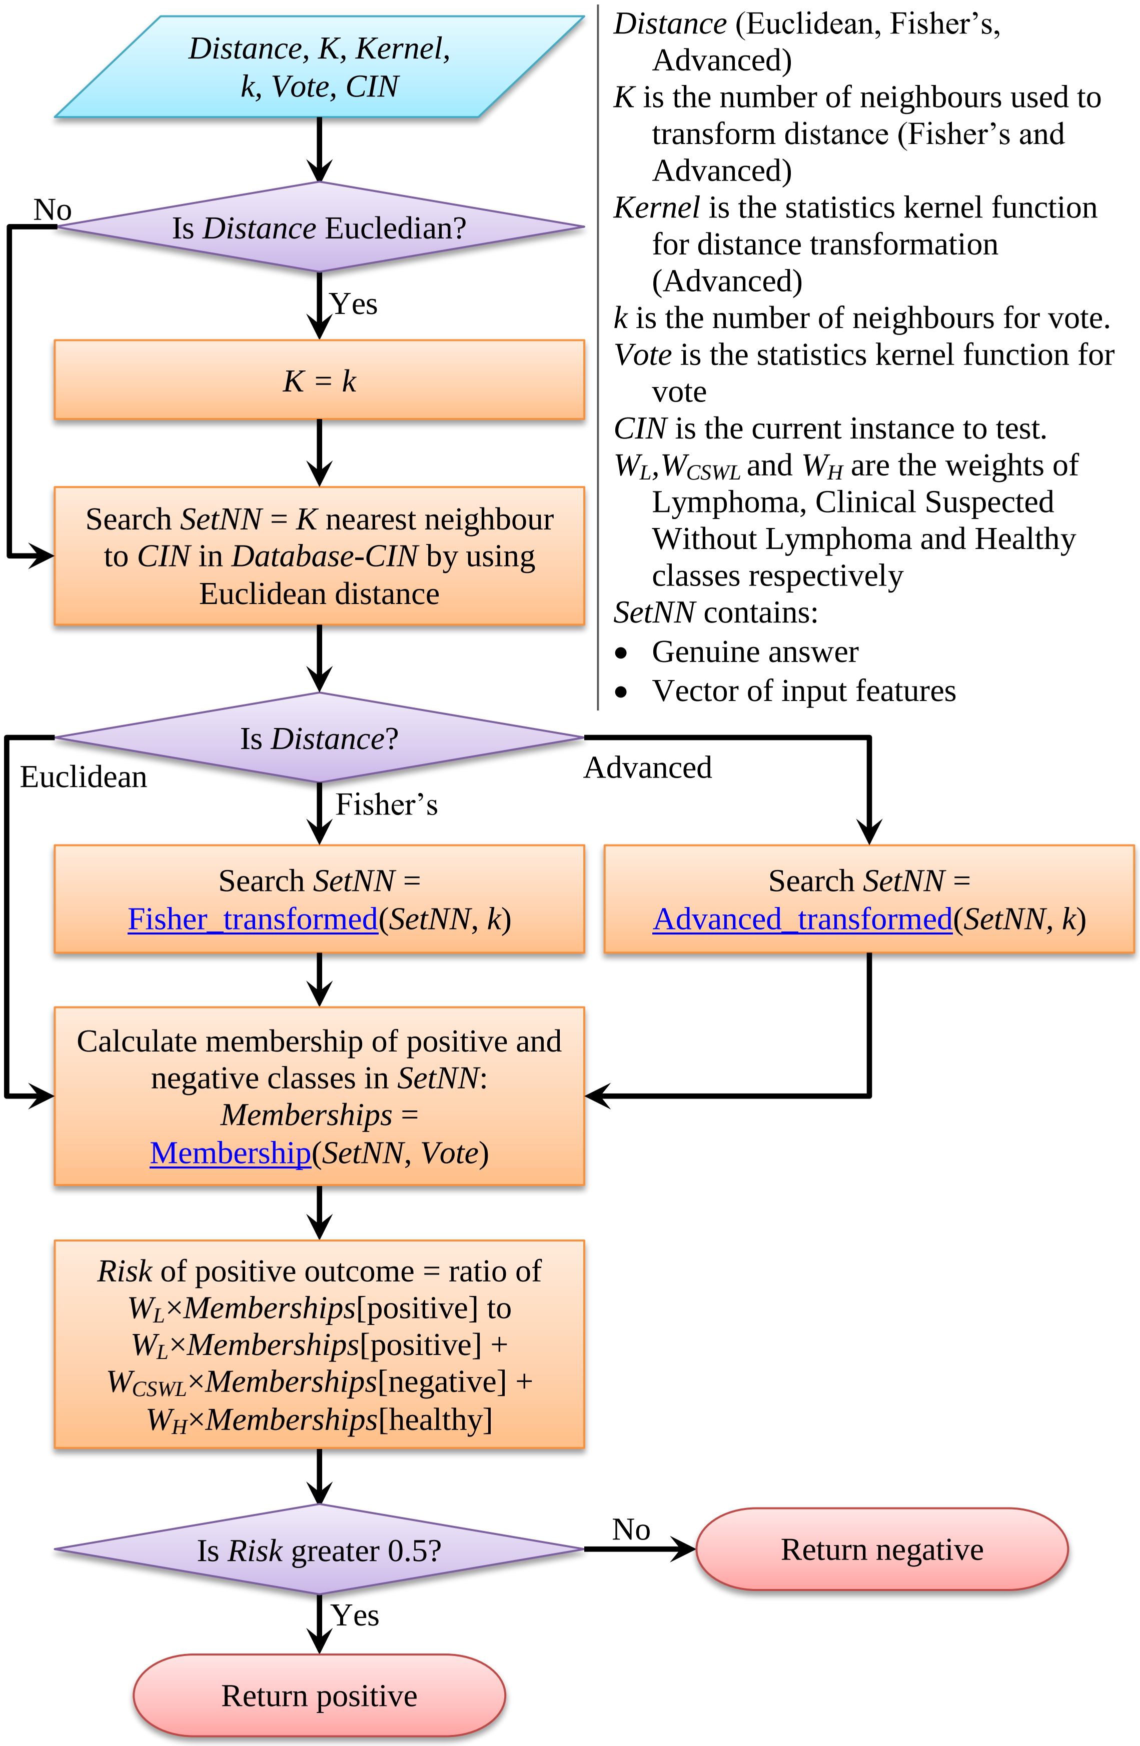


*Distance* (Euclidean, Fisher's, Advanced)

*K* is the number of neighbours used to transform distance (Fisher's and Advanced)

*Kernel* is the statistics kernel function for distance transformation (Advanced)

*k* is the number of neighbours for vote.

*Vote* is the statistics kernel function for vote

*CIN* is the current instance to test.

$W_L$,$W_{CSWL}$ and $W_H$ are the weights of Lymphoma, Clinical Suspected Without Lymphoma and Healthy classes respectively

*SetNN* contains:

- Genuine answer
- Vector of input features

# Fisher's distance transformation Fisher_transformed(*SetNN*, *k*)

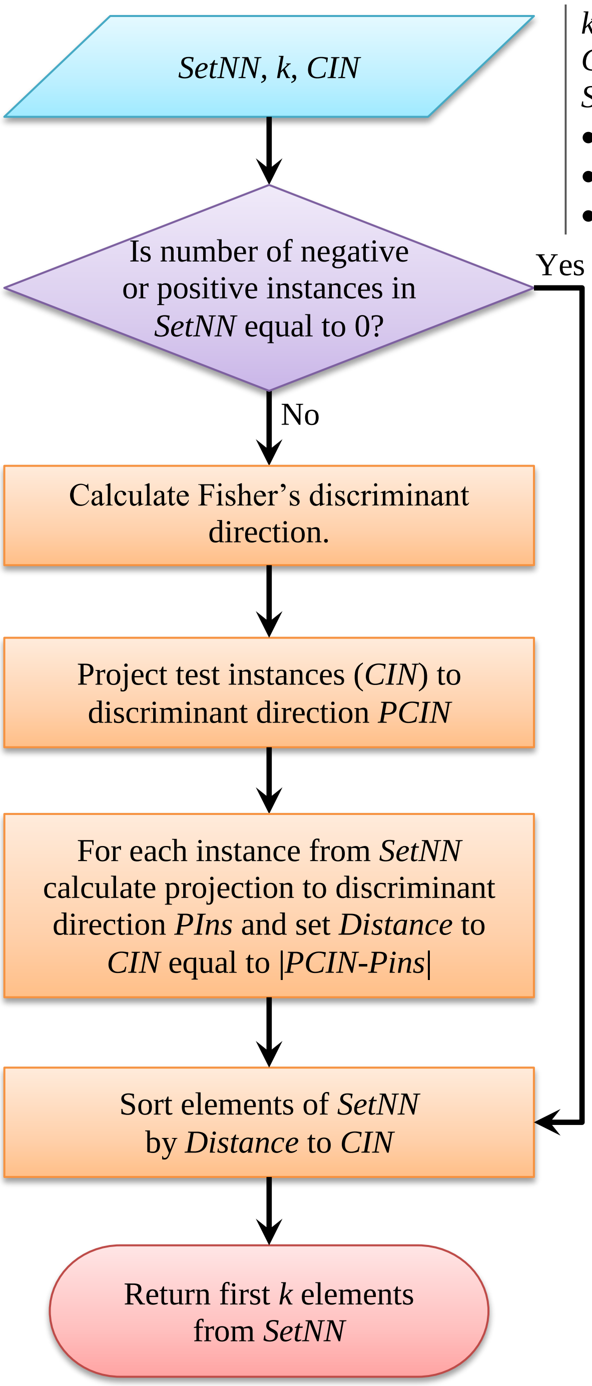


*k* is the number of neighbours for vote
*CIN* is the current instance to test
*SetNN* contains:

- Genuine answer
- Vector of input features
- Distance to *CIN*

# Advanced distance transformation
# Advanced_transformed(*SetNN*, *k*)

*Kernel* is the statistics kernel function for distance transformation
*k* is the number of neighbours for vote.
*CIN* is the current instance to test
*SetNN* contains:

- *i* is number of instance
- Genuine answer $a_i$
- Vector of input features $v_i$
- Distance to *CIN* $d_i$

*P* is the set of positive instances
*N* is set of negative instances

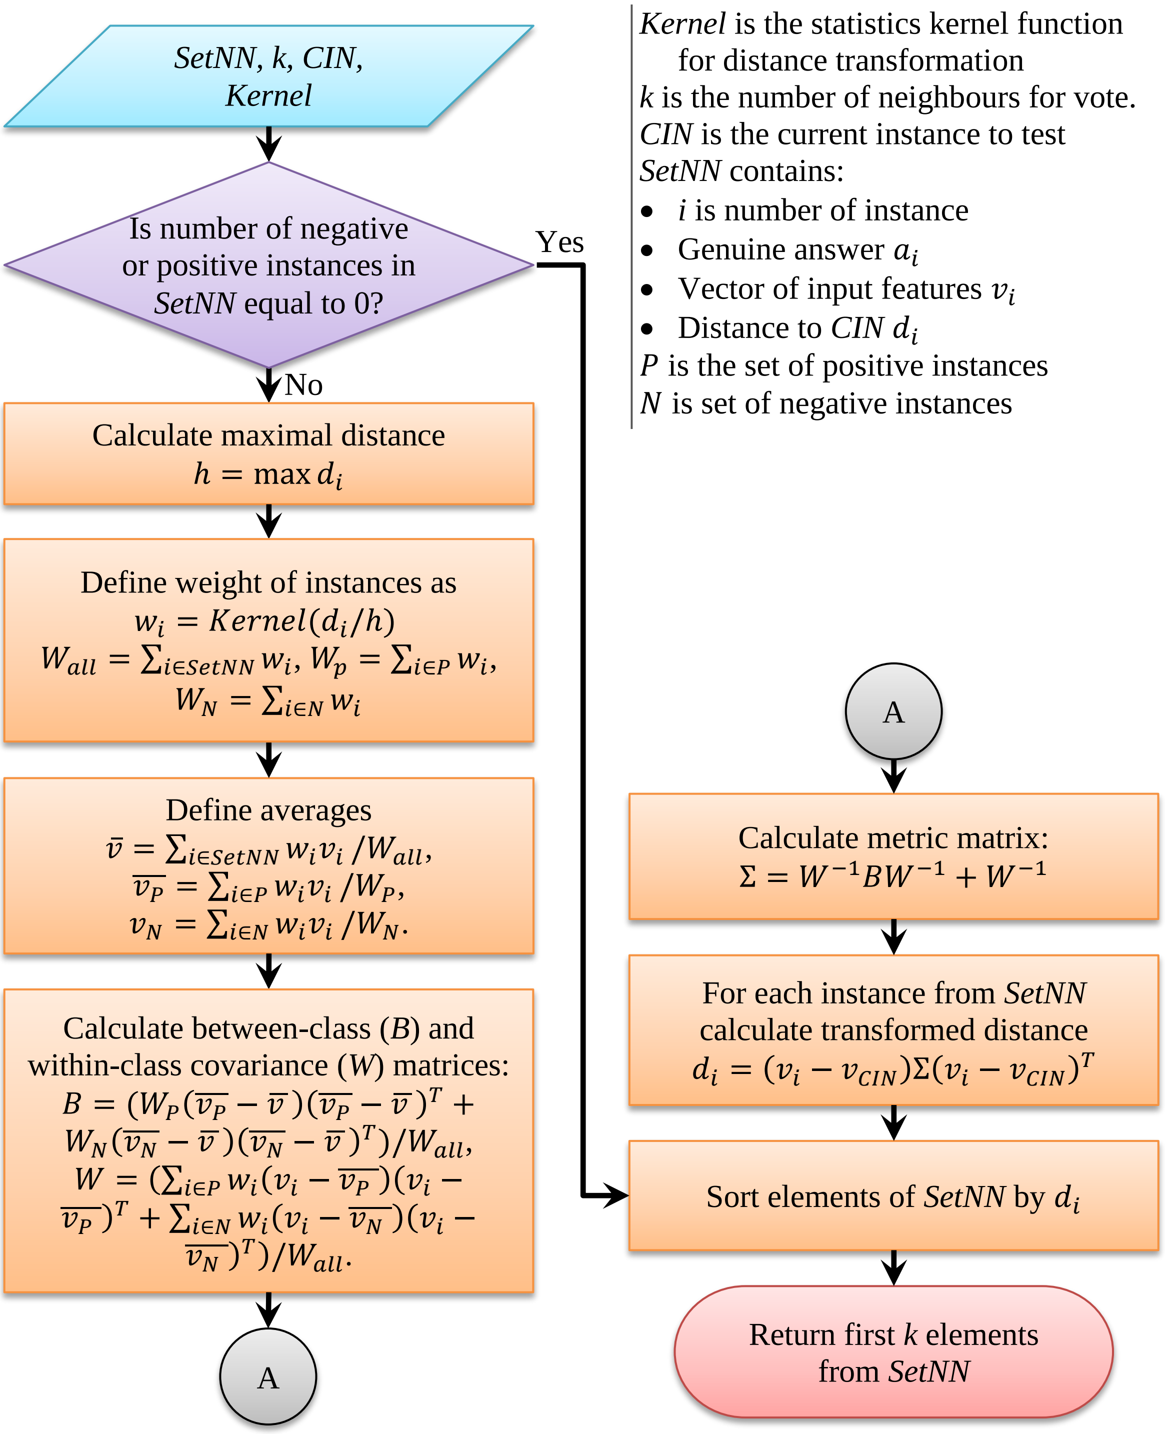

# Calculate membership: Membership(*SetNN*, *Vote*)

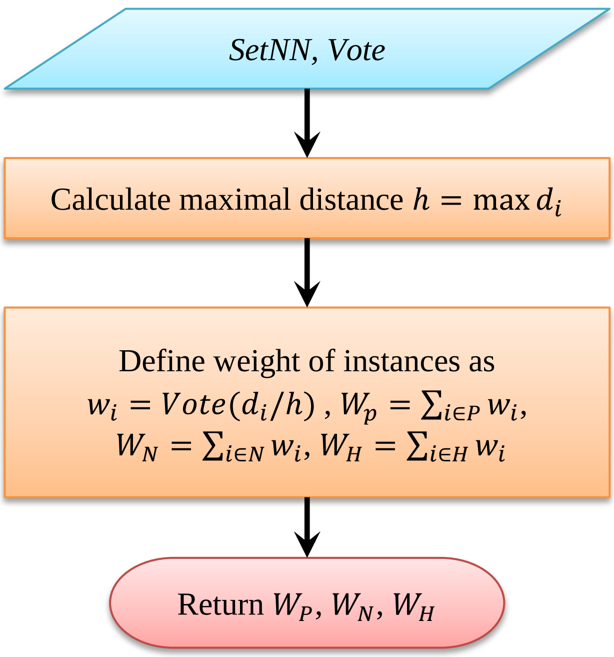


*Vote* is the statistics kernel function for vote

*SetNN* contains:

- $i$ is number of instance
- Genuine answer $a_i$
- Vector of input features $v_i$
- Distance to *CIN* $d_i$

$P$ is the set of positive instances

$N$ is set of negative instances

$H$ is set of healthy instances

## PDFE (probability density function estimation): quality(*Dataset*)

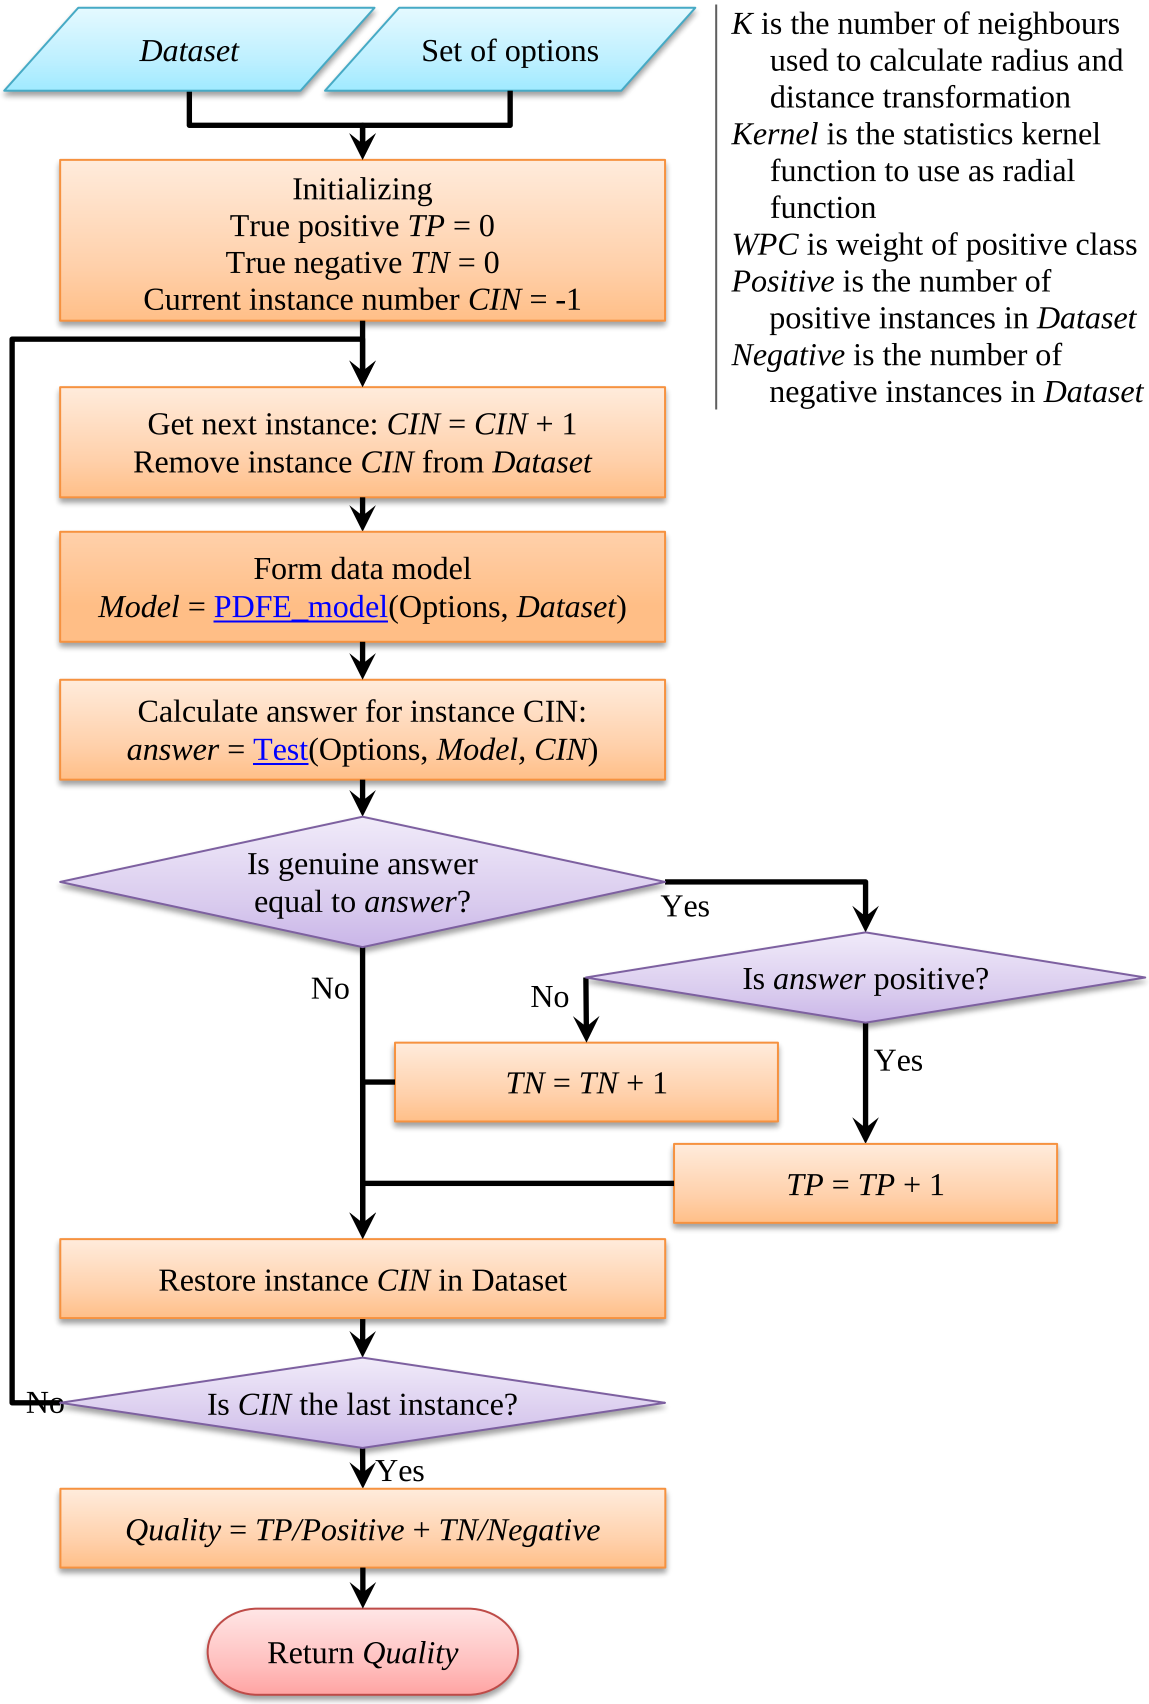


*K* is the number of neighbours used to calculate radius and distance transformation
*Kernel* is the statistics kernel function to use as radial function
*WPC* is weight of positive class
*Positive* is the number of positive instances in *Dataset*
*Negative* is the number of negative instances in *Dataset*

# Fit PDFE: PDFE_model(Options, *Instances*)

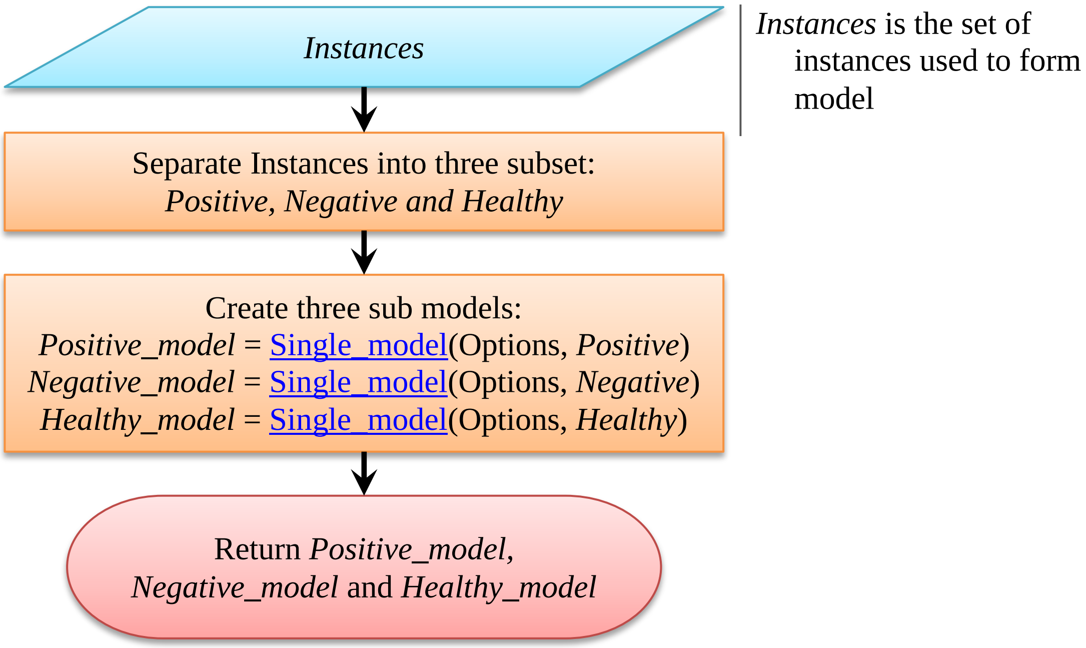

## Form single model Single_model(Options,*Instances*)

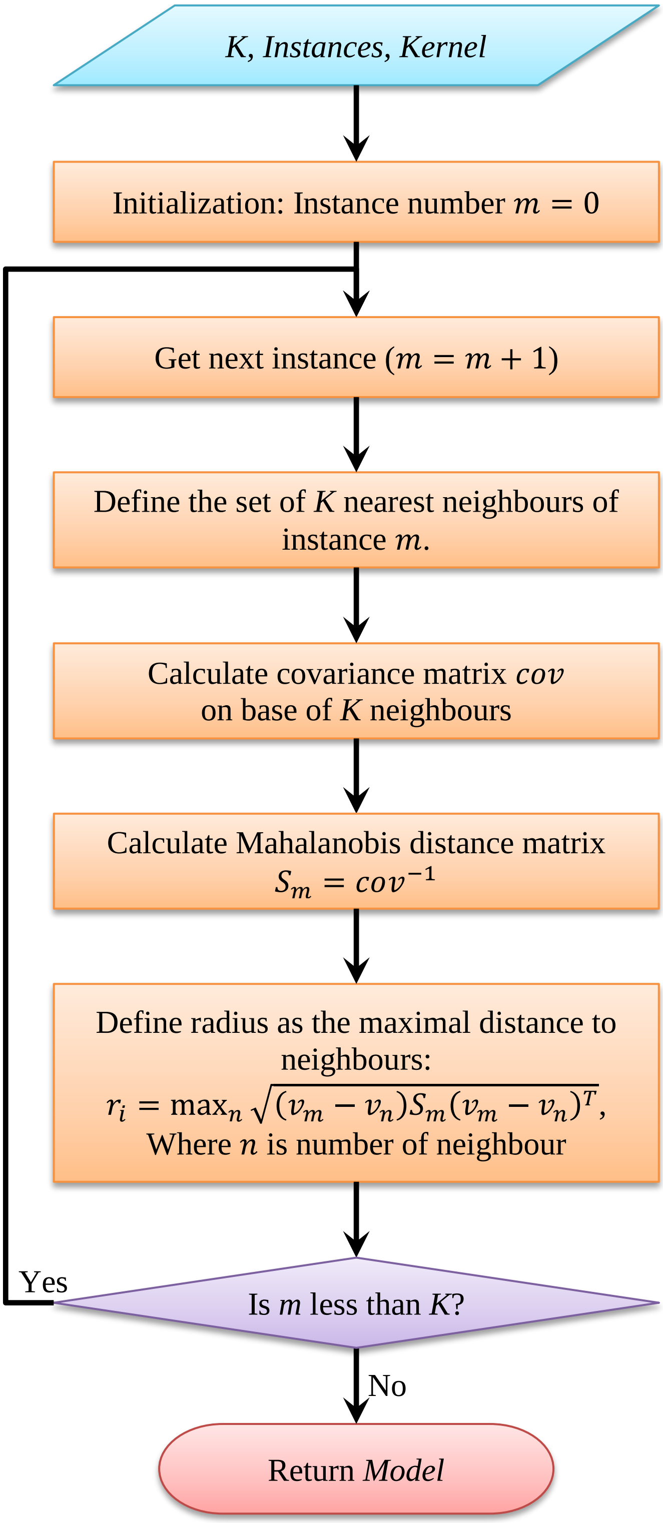


*K* is the number of neighbours used to calculate radius and distance transformation

*Instances* is the set of instances for one class model

*Model* contains for each instance:

- $i$ is number of instance
- *Vector* of input features $v_i$
- $r_i$ is radius
- $S_i$ is Mahalanobis distance matrix

## Test instance: Test(Options, *Model*, *CIN*)

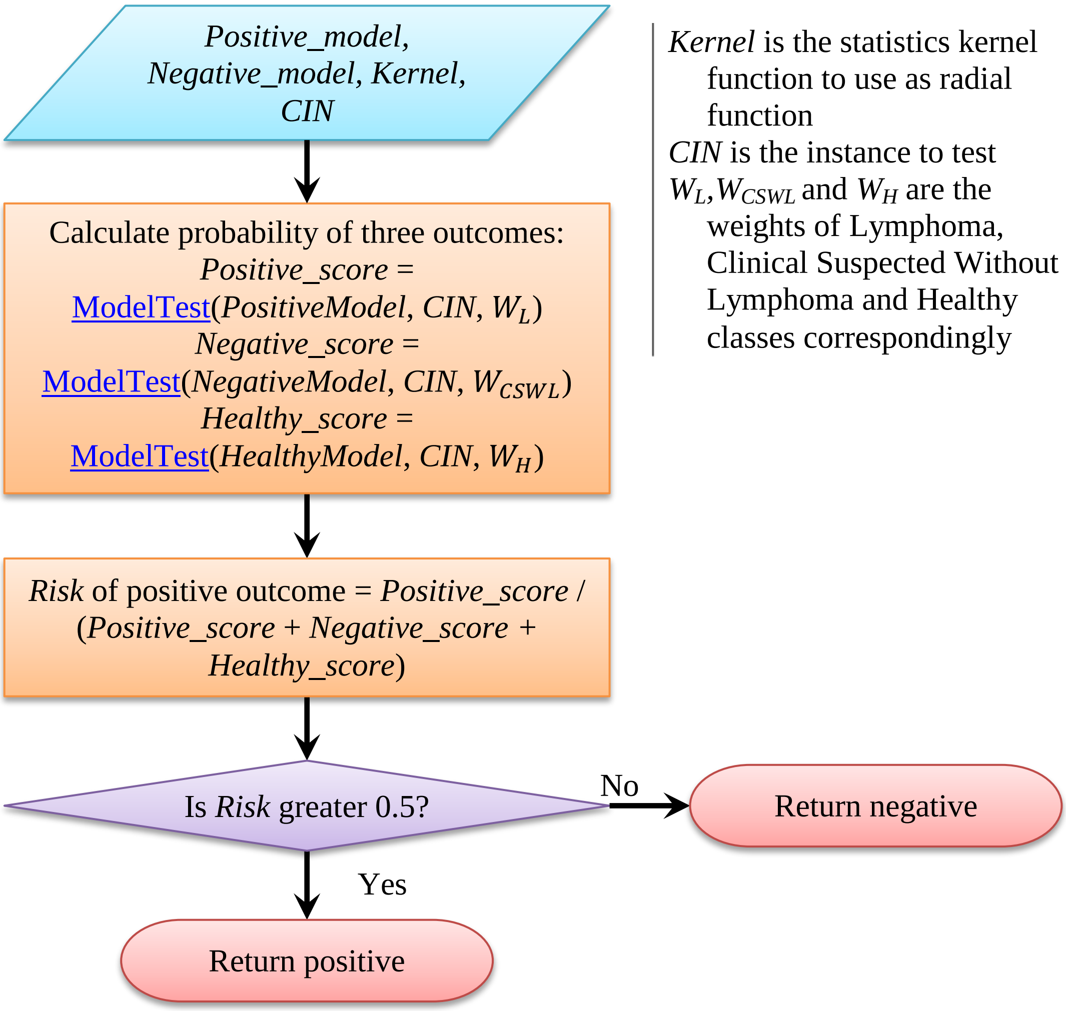

# PDFE one model test: ModelTest(*Model, CIN,W*)

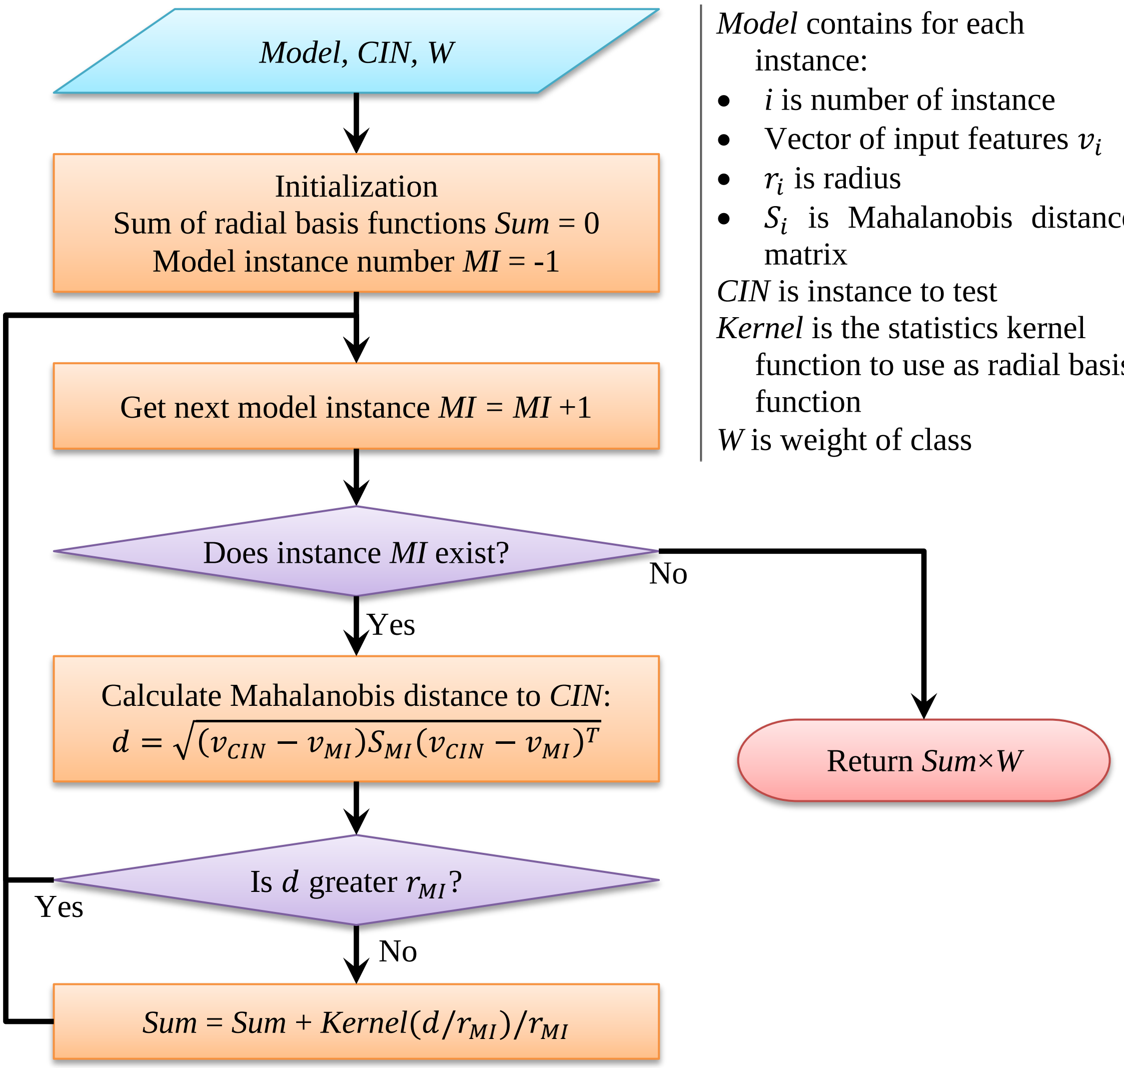


*Model* contains for each instance:

- $i$ is number of instance
- Vector of input features $v_i$
- $r_i$ is radius
- $S_i$ is Mahalanobis distance matrix

*CIN* is instance to test

*Kernel* is the statistics kernel function to use as radial basis function

*W* is weight of class
